# Supplementary material for: On the Complexity of Local Distributed Graph Problems
Source: arXiv:1611.02663 source file (2017-10-28)
Supplement: Supplementary file 1 [file appendix.tex]

\section{Appendix}
Finding a $(\log n, \log n)$-decomposition does not become easier if we consider regular graphs. 
\begin{remark}
\label{remark:regularDecomposition}
Any $(\log n, \log n)$-decomposition algorithm for regular graphs can be turned into a $(\log n, \log n)$-decomposition algorithm for general graphs with the same asymptotic runtime. 
\end{remark}
\begin{proof}[Proof of \Cref{remark:regularDecomposition}]
From  any nonregular graph $G$ we construct a $d$-regular graph $\tilde{G}$ by simply locally appending a graph to every node such that any algorithm in $\tilde{G}$ can be simulated in $G$ with no loss in the number of rounds. Because the virtual of different actual nodes do not have edges  any $(\log n, \log n)$-decomposition of $\tilde{G}$ induces a $(\log n, \log n)$-decomposition  of $G$. The local construction of $\tilde{G}$ works whenever the parameter $d$ is odd, at least as large as the maximum degree $\Delta$ and commonly known by all nodes. E.g., if the maximum degree $\Delta$ is known by every node one can locally simulate $\tilde{G}$ which is obtained by setting $d=2\Delta+1$. Thus a decomposition algorithm for regular graphs induces a decomposition algorithm for general graphs with the same runtime. %

Consider the following procedure to construct the graph $\tilde{G}$: 
Let $v$ be a node with $d(v)\leq \Delta\leq d$ and define $d':=d-d(v)$. If $d'$ is even we add a clique of size $d$, remove  a matching of size $d'/2$ and connect all nodes which take part in the matching with $v$. The degree of $v$ and all newly added nodes will be $d$.
If $d'$  is odd we add a single node $v'$ and connect it with $v$. Now $v$ and $v'$ have an even slack in their degree w.r.t. to $d$-regularity. This slack can be solved independently by the same procedure as in the previous case.

If $d$ is even such a $d$-regular graph cannot be constructed. Simply consider $v$ and $d'=1$ and assume that $d$ is even. Let $H$ be the added graph which makes the graph regular. Assume that $x=|V(H)|$. Then the sum of the degrees of nodes in $H$ is $(x-1)\Delta+\Delta-1$, which is not even, a contradiction.
\end{proof}

In the AMOS decision problem on a graph $G$ every node is equipped with $0$ or $1$ as input and every node has to output either 'yes' or 'no'. If there is at most one node which has $1$ as input the output is admissible if all nodes say $'yes'$. If there is more than one input equal to $1$ the output is admissible if at least one node says 'no'.

\begin{lemma}
For $p^2+p\leq 1$ the AMOS problem is contained in $\randseqloc[0]{p}$ but not in $\seqloc[o(n)]$.
\end{lemma}
